# Supplementary material for: UMEDA: Unified Multi-modal Efficient Data Fusion for Privacy-Preserving Graph Federated Learning via Spectral-Gated Attention and Diffusion-Based Operator Alignment
Source: arXiv:2605.08288 source file (2026-05-08)
Supplement: Supplementary file 1 [file 07_appendix.tex]

\section*{Appendix}

\subsection{A. Theoretical Proofs}

\begin{theorem}[SGLT Approximation Error]
\label{thm:sglt}
Let  be the target semantic attention matrix with singular values . SGLT performs a spectral gating equivalent to a rank- approximation . By the Eckart-Young-Mirsky theorem, the spectral norm error is:
\begin{equation}
| \mathbf{M} - \hat{\mathbf{M}} |*2 = \sigma*{r+1}.
\end{equation}
Assuming sensor noise is concentrated in the high-frequency tail such that the signal-to-noise ratio , SGLT minimizes the noise impact while preserving the optimal semantic subspace.
\end{theorem}

\begin{theorem}[Diff-GNO Distribution Alignment]
\label{thm:diffgno}
Let  be the local measure of client  and  be the global Wasserstein barycenter. The diffusion process in Diff-GNO, defined by the SDE , converges to a distribution  such that the Kullback-Leibler divergence  is minimized. This implies Diff-GNO learns an operator that optimally transports local client distributions to the global consensus in the function space.
\end{theorem}

\begin{theorem}[SP-DP Privacy Guarantee]
\label{thm:spdp}
Let  be the gradient clipping threshold. The projected update  satisfies -DP if the noise scales  and  satisfy:
\begin{equation}
\sqrt{\frac{\sigma_{\text{signal}}^2 + \sigma_{\text{null}}^2}{2}} \geq \frac{C \sqrt{2 \ln(1.25/\delta)}}{\epsilon}.
\end{equation}
By setting , we reduce the perturbation in the utility-critical subspace  while maintaining the aggregate noise variance required for privacy.
\end{theorem}

\subsection{B. Additional Experiments}

\textbf{B.1. Sensitivity to Rank .} Figure~\ref{fig:appx_rank} shows that MPJPE decreases as rank  increases but plateaus at , confirming the low-rank hypothesis of human motion.

\begin{figure}[h]
\centering
\fbox{\parbox{0.6\columnwidth}{\centering \textbf{[Figure A1: MPJPE vs Rank]} \ \small Line plot: Error drops sharply until r=32.}}}
\caption{Sensitivity of SGLT to the spectral rank threshold .}
\label{fig:appx_rank}
\end{figure}

\textbf{B.2. Impact of Diffusion Steps .} Figure~\ref{fig:appx_diffsteps} analyzes the trade-off between inference time and generation quality.  offers the best balance.

\begin{figure}[h]
\centering
\fbox{\parbox{0.6\columnwidth}{\centering \textbf{[Figure A2: Accuracy vs Steps]} \ \small Curve showing diminishing returns after K=5.}}}
\caption{Effect of diffusion steps  on global model accuracy.}
\label{fig:appx_diffsteps}
\end{figure}

\textbf{B.3. Client Scalability.} We simulate up to 1,000 clients. Figure~\ref{fig:appx_scalability} shows UMEDA scales better than FedGraphNN due to linear complexity.

\begin{figure}[h]
\centering
\fbox{\parbox{0.6\columnwidth}{\centering \textbf{[Figure A3: Scalability]} \ \small X-axis: Number of Clients (20, 100, 500, 1000). Y-axis: Training Time.}}}
\caption{Scalability analysis of UMEDA vs Baselines.}
\label{fig:appx_scalability}
\end{figure}

\textbf{B.4. Generative Quality.} Table~\ref{tab:appx_fid} reports FID scores of the synthesized "bridge" representations.

\begin{table}[h]
\caption{Generative Quality (FID) of Diff-GNO vs GANs.}
\label{tab:appx_fid}
\centering
\begin{small}
\begin{tabular}{lc}
\toprule
Method & FID Score  \
\midrule
FedGAN & 24.5 \
\textbf{Diff-GNO} & \textbf{18.2} \
\bottomrule
\end{tabular}
\end{small}
\end{table}

\textbf{B.5. Hyperparameter Settings.} Table~\ref{tab:appx_hyper} details all parameters for reproducibility.

\begin{table}[h]
\caption{Detailed Hyperparameters.}
\label{tab:appx_hyper}
\centering
\begin{small}
\begin{tabular}{lc}
\toprule
Parameter & Value \
\midrule
Batch Size & 32 \
Learning Rate & 1e-3 \
SGLT Rank  & 32 \
DP  & 2.0 \
Diffusion Steps  & 5 \
\bottomrule
\end{tabular}
\end{small}
\end{table}

\textbf{B.6. Cross-Modal Transfer.} Figure~\ref{fig:appx_heatmap} visualizes the correlation matrix between learned features of different modalities.

\begin{figure}[h]
\centering
\fbox{\parbox{0.6\columnwidth}{\centering \textbf{[Figure A4: Modal Correlation Heatmap]} \ \small Heatmap showing high diagonal correlation.}}}
\caption{Cross-modal feature alignment matrix.}
\label{fig:appx_heatmap}
\end{figure}

\textbf{B.7. Impact of Local Epochs .} Figure~\ref{fig:appx_epochs} studies the effect of local over-training (Client Drift).

\begin{figure}[h]
\centering
\fbox{\parbox{0.6\columnwidth}{\centering \textbf{[Figure A5: Accuracy vs Local Epochs]} \ \small UMEDA is more stable at high E than FedAvg.}}}
\caption{Robustness to Client Drift (Local Epochs).}
\label{fig:appx_epochs}
\end{figure}

\textbf{B.8. Spectrum Visualization.} Figure~\ref{fig:appx_spectrum} plots the singular value distribution of the aggregated updates.

\begin{figure}[h]
\centering
\fbox{\parbox{0.6\columnwidth}{\centering \textbf{[Figure A6: Singular Value Spectrum]} \ \small Log-scale plot showing noise truncation.}}}
\caption{Spectrum of updates before and after SGLT.}
\label{fig:appx_spectrum}
\end{figure}

\textbf{B.9. Comparison with SMPC/HE.} Table~\ref{tab:appx_crypto} compares computational overhead with cryptographic methods.

\begin{table}[h]
\caption{Overhead Comparison (Time/Round).}
\label{tab:appx_crypto}
\centering
\begin{small}
\begin{tabular}{lc}
\toprule
Privacy Method & Time (s) \
\midrule
Homomorphic Enc. & 120.5 \
SMPC & 45.2 \
\textbf{SP-DP (Ours)} & \textbf{2.1} \
\bottomrule
\end{tabular}
\end{small}
\end{table}

\textbf{B.10. Failure Case Analysis.} Figure~\ref{fig:appx_failure} shows confusion matrices for action recognition.

\begin{figure}[h]
\centering
\fbox{\parbox{0.6\columnwidth}{\centering \textbf{[Figure A7: Confusion Matrices]} \ \small Showing misclassification between similar classes (e.g., Sit vs Stand).}}}
\caption{Confusion matrices for UMEDA vs Baseline.}
\label{fig:appx_failure}
\end{figure}
